# Supplementary material for: Rank-one matrix estimation: analysis of algorithmic and information theoretic limits by the spatial coupling method
Source: arXiv:1812.02537 source file (2018-12-06)
Supplement: Supplementary file 1 [file appendix_Mmse.tex]

\section{Connection between matrix and vector MMSE} \label{app:Mmmse}
In this appendix we prove Lemma \ref{lemma:Mmmse} that links the matrix MMSE to the signal (or vector) MMSE.

Consider the perturbed model associated with the Hamiltonian \eqref{eq:perturbed_hamiltonian}. As in section~\ref{subsec:concentration1}, denote $\langle A(\bX) \rangle_h$ the expectation w.r.t the posterior associated with this Hamiltonian, see \eqref{eq:posterior_partition}. For this model, the matrix and vector MMSE are
\begin{align}
{\rm Mmmse}_{n,h} &\defeq \frac{1}{n^2}\mathbb{E}_{\bS, \bW}\Big[ \bigl\| \bS\bS^{\intercal} - \langle\bX\bX^{\intercal}\rangle_h\bigr\|_{\rm F}^2 \Big], \label{eq:matrix_mmse}\\ 
{\rm Vmmse}_{n,h} &\defeq \frac{1}{n}\mathbb{E}_{\bS, \bW}\Big[ \bigl\| \bS - \langle\bX\rangle_h\bigr\|_{2}^2 \Big]. \label{eq:vector_mmse}
\end{align}
Expanding the Frobenius norm in (\ref{eq:matrix_mmse}) yields
\begin{align}
{\rm Mmmse}_{n,h} &= \frac{1}{n^2}\mathbb{E}_{\bS, \bW}\Big[ \sum_{i,j=1}^n ( S_i S_j - \langle X_i X_j\rangle_h)^2 \Big] =\frac{1}{n^2}\mathbb{E}_{\bS, \bW}\Big[ \sum_{i,j=1}^n  S_i^2 S_j^2 - \langle X_i X_j\rangle_h^2 \Big] \nonumber \\
&= \mathbb{E}_{\bS}\Big[\Big(\frac{1}{n}\sum_{i=1}^n S_i^2\Big)^2 \Big] - \frac{1}{n^2} \sum_{i,j=1}^n \mathbb{E}_{\bS, \bW}[\langle X_i X_j \rangle_h^2], 
\end{align}
where the second equality follows from $\mathbb{E}_{\bS, \bW}[\langle X_i X_j\rangle_h^2]=\mathbb{E}_{\bS, \bW}[ S_i S_j \langle X_i X_j\rangle_h]$, implied by the Nishimori condition \eqref{eq:nishCond}. Similarly, (\ref{eq:vector_mmse}) simplifies to
\begin{align}
{\rm Vmmse}_{n,h} = v - \frac{1}{n}\sum_{i=1}^n \mathbb{E}_{\bS, \bW}[\langle X_i\rangle_h^2 ]. 
\end{align}
Define the following quantities
\begin{align}
\mathcal{A}_{n} &\defeq  \mathbb{E}_{\bS}\Big[\Big(\frac{1}{n}\sum_{i=1}^n S_i^2\Big)^2 \Big] - v^2, \\
\mathcal{B}_{n,h} &\defeq \frac{1}{n^2} \sum_{i,j=1}^n \Big(\mathbb{E}_{\bS, \bW}[ \langle X_i X_j \rangle_h^2 ] - \mathbb{E}_{\bS, \bW}[\langle X_i \rangle_h^2 ]\mathbb{E}_{\bS, \bW}[\langle X_j \rangle_h^2 ]\Big).\label{eq:Mmmse_Vmmse_diff_1}
\end{align}
Then one obtains for $a>\epsilon>0$
\begin{align}
\int_\epsilon^a dh \Big( {\rm Mmmse}_{n,h} - ( v^2 - (v - {\rm Vmmse}_{n,h})^2 )\Big) = (a-\epsilon)\mathcal{A}_n - \int_\epsilon^a dh \mathcal{B}_{n,h}. \label{eq:Mmmse_Vmmse_diff}
\end{align}
Note that as the signal components $\{S_i\}$ are i.i.d, then $\lim_{n \to\infty}\mathcal{A}_n = 0$ by the law of large numbers. Remains to show that the same is true for the remaining term. Recall the overlap is defined as $q(\bX,\bS) \defeq \sum_{i=1}^n S_iX_i/n$. The identities $\mathbb{E}_{\bS, \bW}[\langle X_i \rangle_h^2 ] = \mathbb{E}_{\bS, \bW}[S_i\langle X_i \rangle_h ]$ and $\mathbb{E}_{\bS, \bW}[\langle X_i X_j\rangle_h^2]=\mathbb{E}_{\bS, \bW}[ S_i S_j \langle X_i X_j\rangle_h]$, due to the Nishimori condition, yield
\begin{align}
\mathcal{B}_{n,h} &= \mathbb{E}_{\bS, \bW}[ \langle q^2\rangle_h ] -  \mathbb{E}_{\bS, \bW}[\langle q \rangle_h]^2 \nonumber \\
&=  (\mathbb{E}_{\bS, \bW}[ \langle q^2\rangle_h ] - \mathbb{E}_{\bS, \bW}[ \langle q\rangle_h^2 ]) + (\mathbb{E}_{\bS, \bW}[\langle q \rangle_h^2 ] - \mathbb{E}_{\bW}[\mathbb{E}_{\bS}[ \langle q\rangle_h ]^2] )\nonumber \\
&\ \ \ +  ( \mathbb{E}_{\bW}[\mathbb{E}_{\bS}[ \langle q\rangle_h ]^2] -\mathbb{E}_{\bS, \bW}[\langle q \rangle_h ]^2  )  \nonumber\\
&=   \mathbb{E}_{\bS,\bW}[ \langle (q - \langle q \rangle_h )^2\rangle_h ] + \mathbb{E}_{\bS,\bW}[ ( \langle q\rangle_h -\mathbb{E}_{\bS}[\langle q\rangle_h])^2] + \mathbb{E}_{\bW}[(\mathbb{E}_{\bS}[\langle q \rangle_h ] - \mathbb{E}_{\bS,\bW}[\langle q \rangle_h ])^2 ]   \nonumber \\
&\eqdef  \mathcal{B}_{n,h}^{(1)} + \mathcal{B}_{n,h}^{(2)} + \mathcal{B}_{n,h}^{(3)}.
\end{align}
Each term $\mathcal{B}_{n,h}^{(i)}$ can be interpreted as overlap fluctuations due to a different source of randomness. The concentration properties shown in Appendix~\ref{app:concentration} are useful here to show the desired result. Indeed, Lemma~\ref{lemma:concentration_q} applied to the first term, Lemma~\ref{lemma:concentration_meanq} to the second and Lemma~\ref{lemma:concentration_mean2} applied to the third respectively imply all together that 
\begin{align}
\lim_{n\to\infty}\int_\epsilon^a dh \mathcal{B}_{n,h} = 0.
\end{align}
Recall that \eqref{eq:matrix_mmse}, \eqref{eq:vector_mmse} are functions of the noise variance. Combining this last equality with the result on the limit of $\mathcal{A}_n$ allows to assert using \eqref{eq:Mmmse_Vmmse_diff}
\begin{align}
&\lim_{n\to\infty}\int_\epsilon^a dh \Big( {\rm Mmmse}_{n,h}(\Delta^{-1}) - ( v^2 - (v - {\rm Vmmse}_{n,h}(\Delta^{-1}))^2 )\Big)=0.
\end{align}
We now need the following technical lemmas.
\begin{lemma}\label{lemma:cond_redices_MMSE}
Conditionning reduces the MMSE, that is for any jointly distributed $\bX$ and $\bY$,
\begin{align}
\mathbb{E}_{\bY}[{\rm mmse}(\bX|\bY)] \le {\rm mmse}(\bX).
\end{align}
\end{lemma}
\begin{proof}
Despite the proof is done in [\cite{5730572}], we give here an alternative and more computationnal one for sake of completeness. We prove it here in full generality, and the results applies to both the vector and matrix MMSE. Assume some observation $\bW$ is accessible about $\bS$ (with $\mathbb{E}_\bS[S^2]=v$). Furthermore, assume that there exists $\bY$ that is jointly distributed with $\bS$ (and thus with $\bX$ too). Using the identity $\mathbb{E}_{\bW,\bS}[S_i\mathbb{E}[X_i|\bW,\bY]] = \mathbb{E}_{\bW,\bS}[\mathbb{E}[X_i|\bW,\bY]^2]$ due to the Nishimori identity, one obtains
\begin{align}
\mathbb{E}_{\bY}[{\rm mmse}(\bX|\bY)] &= v - \mathbb{E}_{\bS,\bW,\bY}[\mathbb{E}[\bX|\bW,\bY]^2] \le v - \mathbb{E}_{\bS,\bW}[\mathbb{E}_\bY[\mathbb{E}[\bX|\bW,\bY]]^2] \nonumber \\
&= v - \mathbb{E}_{\bS,\bW}[\mathbb{E}[\bX|\bW]^2] = {\rm mmse}(\bX),
\end{align}
where the inequality is due to the convexity of the square.
\end{proof}
\begin{lemma} \label{lemma:existence_limits_mmse}
The limits of \eqref{eq:matrix_mmse} and \eqref{eq:vector_mmse} exist: 
\begin{align}
\lim_{n\to\infty} {\rm Mmmse}_{n,h}(\Delta^{-1})&={\rm Mmmse}_{h}(\Delta^{-1}), \\
\lim_{n\to\infty} {\rm Vmmse}_{n,h}(\Delta^{-1})&= {\rm Vmmse}_{h}(\Delta^{-1}).
\end{align}
\end{lemma}
\begin{proof}
We follow an argument given in [\cite{6875223}]. Denote ${\rm mmse}({\rm snr}_n| \bW_n)\defeq {\rm Vmmse}(\Delta^{-1})$ the vector MMSE \eqref{eq:vector_mmse} where $\bs$ has $n$ components, the observation matrix $\bW_n$ has dimension $n\times n$ and the signal-to-noise in the model \eqref{eq:mainProblem} is readily equal to ${\rm snr}_n = v^2/(n\Delta)$. Denote $\bW_{n-1}$ the $(n-1)\times (n-1)$ first principal submatrix of $\bW_n$, $\bar \bW_{n-1}$ the remaining entries of $\bW_n$ not in $\bW_{n-1}$. We have that
\begin{align}
{\rm mmse}({\rm snr}_n| \bW_n) = {\rm mmse}({\rm snr}_n| \bW_{n-1}, \bar \bW_{n-1}) \le {\rm mmse}({\rm snr}_{n-1}| \bW_{n-1}),
\end{align}
using Lemma~\ref{lemma:cond_redices_MMSE}. Now note that ${\rm snr}_{n-1} = {\rm snr}_{n}(1-n^{-1})^2$. Furthermore, it is proven in [\cite{5730572}] that the MMSE function is monotone decreasing in the ${\rm snr}$. Thus 
\begin{align}
{\rm mmse}({\rm snr}_n| \bW_n) \le {\rm mmse}({\rm snr}_{n-1}| \bW_{n-1}) \le {\rm mmse}({\rm snr}_{n}| \bW_{n-1}),
\end{align}
which proves that the MMSE is a monotone decreasing sequence. Furthermore, it is bounded and thus have a limit as $n\to\infty$.
\end{proof}
Thus $\lim_{n\to\infty}( {\rm Mmmse}_{n,h}(\Delta^{-1}) - ( v^2 - (v - {\rm Vmmse}_{n,h}(\Delta^{-1}))^2 ))$ is vanishing for almost every $h\in[\epsilon, a]$. In order to get back the original model, we need to take the limit $h\to 0$. To do so, let $\epsilon \to 0$, then for a given noise variance $\Delta$ choose a sequence $\{h_n\}$ such that $\lim_{n\to \infty}$
