# Supplementary material for: Rank-one matrix estimation: analysis of algorithmic and information theoretic limits by the spatial coupling method
Source: arXiv:1812.02537 source file (2018-12-06)
Supplement: Supplementary file 2 [file appendix_concentration.tex]

\section{Concentration of the overlap} \label{app:concentration}
In this appendix, we prove useful concentration properties for the overlap $q = q(\bx,\bs) \defeq 1/n \sum_{i=1} s_ix_i$ between $\bs$ and $\bx$, that turn out to be necessary to show formula ?? linking the signal and matrix MMSE. Three distinct concentrations properties will be shown, that all use different proof techniques depending on the nature of the randomness that is considered for the concentration.
\subsection{Concentration of $q$ on $\langle q \rangle_{h}$} \label{subsec:concentration1}
The first step is to show the concentration of the overlap $q$ around its expectation value w.r.t the posterior distribution at fixed disorder realization. The disorder refers to the signal and noize realizations, borrowing vocabulary of statistical mechanics. Consider a \emph{perturbed} system with the following Hamiltonian
\begin{align}\label{eq:perturbed_hamiltonian}
\mathcal{H}(\bx, \bs,\bz,h) &= \frac{1}{\Delta} \sum_{1 \le i\le j\le n}\bigg[ \frac{x_{i}^2x_{j}^2}{2n} -  \frac{s_{i}s_{j}x_{i}x_{j}}{n} - \frac{x_{i}x_{j}z_{i j} \sqrt{\Delta}}{\sqrt{n}} \bigg] + h \sum_{i=1}^n s_ix_i,
\end{align}
where a perturbation term $h \sum_{i=1}^n s_ix_i$ is added to the Hamiltonian $\mathcal{H}(\bx, \bs,\bz,h=0)$ of the underlying system \eqref{eq:mainProblem}. However, for some technical reasons that will become clear in the sequel, we work with the perturbed system (\ref{eq:perturbed_hamiltonian}) and then let $h \rightarrow 0$ at the end of the analysis. Furthermore, call $\mathcal{Z}(\bs,\bz, h)=\int d\bx P_0(\bx)\exp(-\mathcal{H}(\bx,\bs,\bz, h))$ the partition function of the perturbed system and $f(\bs,\bz,h) = -\ln(\mathcal{Z}(\bs,\bz,h) )/n$ the associated free energy at fixed disorder realization. Moreover, we denote by $\langle A({\bX}) \rangle_{h}$ the expectation w.r.t the posterior distribution associated with $\mathcal{H}(\bx,\bs,\bz,h)$, see \eqref{eq:posterior_partition}. Note the the perturbation term has been chosen so that the following lemma holds.
\begin{lemma}\label{lemma:perturbed_energy_concave}
The free energy $f(\bs,\bz,h)$ is concave in $h$.
\end{lemma}
\begin{proof}
By using the dominated convergence theorem, one obtains the following
\begin{align}
\label{eq:perturbed_energy_derivative1}
\frac{df(\bs,\bz,h)}{dh} &=  \langle q \rangle_{h}, \\
\label{eq:perturbed_energy_derivative2}
\frac{d^2f(\bs,\bz,h)}{dh^2} &= - n ( \langle q^2 \rangle_{h} - \langle q \rangle_{h}^2 ) \le 0,
\end{align}
where $\langle q \rangle_{h} = \langle q(\bX, \bs) \rangle_{h}$.
\end{proof}
We can now show the first concentration property of the overlap $q$.
\begin{lemma}[Concentration of $q$]\label{lemma:concentration_q}
For any $a >\epsilon>0$ fixed
\begin{align}
\int_{\epsilon}^{a} dh \mathbb{E}_{{\bS}, {\bZ}} [\langle (q - \langle q \rangle_{h} )^2 \rangle_{h}] = \mathcal{O}(1/n).
\end{align}
\end{lemma}
\begin{proof}
Let us evaluate the integral
\begin{align}
\int_{\epsilon}^{a} dh \mathbb{E}_{{\bS}, {\bZ}} [\langle (q - \langle q \rangle_{h} )^2 \rangle_{h}]
&= \int_{\epsilon}^{a} dh \mathbb{E}_{{\bS}, {\bZ}}[ \langle q^2 \rangle_{h} - \langle q \rangle_{h}^2 ] \nonumber\\
&= - \frac{1}{n} \int_{\epsilon}^{a} dh \frac{d^2\,\mathbb{E}_{{\bS}, {\bZ}}[f({\bS},{\bZ},h)]}{dh^2} \nonumber\\
&= \frac{1}{n} \Big( \frac{d\,\mathbb{E}_{{\bS}, {\bZ}}[f({\bS},{\bZ},h)]}{dh}\Big|_{\epsilon} - \frac{d\,\mathbb{E}_{{\bS}, {\bZ}}[f({\bS},{\bZ},h)]}{dh}\Big|_{a}  \Big),
\end{align}
where the second equality follows from (\ref{eq:perturbed_energy_derivative2}) and the dominated convergence theorem. We now show that the derivatives of the free energy are both $\mathcal{O}(1)$. Indeed
\begin{align}
\frac{d\,\mathbb{E}_{{\bS}, {\bZ}}[f({\bS},{\bZ},h)]}{dh} =  \frac{1}{n} \sum_{i=1}^n \mathbb{E}_{{\bS}, {\bZ}}[ S_i\langle X_i \rangle_{h}] \le \mathbb{E}_{{\bS}}[S^2 ] = v,
\end{align} 
where the last inequality is obtained by Cauchy-Schwarz inequality and using the Nishimori condition. Finally, as by assumption the prior distribution has bounded second moment $v$, the result follows.
\end{proof} 
\subsection{Concentration of $\langle q\rangle_h$ on $\mathbb{E}_{{\bS}}[\langle q \rangle_h]$} \label{subsec:concetration2}
%
% Denote the Hamiltonian associated with the underlying system \eqref{eq:mainProblem} as $\mathcal{H}(\bx,\bs, \bz) = \mathcal{H}(\bx,\bs,\bz,h=0)$, where $\mathcal{H}(\bx,\bs,\bz,h)$ is given by \eqref{eq:perturbed_hamiltonian}. For this section denote $\langle \cdot \rangle$ as the expectation w.r.t the posterior associated with $\mathcal{H}(\bx,\bs, \bz)$. Furthermore, call $\mathcal{Z}(\bs,\bz)=\int d\bx P_0(\bx)\exp(-\mathcal{H}(\bx,\bs,\bz))$ the partition of the underlying system and $f(\bs,\bz) = -\ln(\mathcal{Z}(\bs,\bz) )/n$ the associated free energy at fixed signal and noize realizations. 
The next result we need is the concentration of $\langle q \rangle_h$, that is computed at fixed disorder realization, around its expectation w.r.t the signal realization $\mathbb{E}_{{\bS}}[\langle q \rangle]$. The proof strategy is based on a powerful concentration inequality for functions of random variables verifying the so-called bounded difference property [\cite{McDiarmid}]. See also [\cite{boucheron2004concentration}] for a very nice and complete review on concentration inequalities. As in the previous section, the concentration of the averaged overlap will be obtained by studying the free energy of the perturbed system. Let us start by showing that this free energy verifies the bounded difference property. Call a perturbed version of the signal $\tilde \bs^{(i)} \defeq [s_1, s_2, \ldots, s_{i-1}, \tilde s_i, s_{i+1},\ldots ,s_n]$, where the $i^{th}$ signal component is modified w.r.t $\bs$. 
\begin{lemma}[Bounded difference property] \label{lemma:bounded_diff_prop}
Fix a noize realization $\bz$. The free energy of the perturbed system verifies the bounded difference property w.r.t the signal, that is
\begin{align}
|f(\bs,\bz,h) - f(\tilde \bs^{(i)},\bz,h)| = \mathcal{O}(1/n) \ \forall \ i \in \{1:n\}.
\end{align}
\end{lemma}
\begin{proof}
Let us focus on a modification of the first component of the signal, but all the following steps hold perturbing any component $i \in\{1:n\}$. We start evaluating the difference between the perturbed Hamiltonian \eqref{eq:perturbed_hamiltonian} evaluated at $\bs$ and $\tilde\bs^{(1)}$.
\begin{align}
\delta \mathcal{H}(\bx,\tilde \bs^{(1)}, \bs,h) \defeq \mathcal{H}(\bx,\bs, \bz,h) - \mathcal{H}(\bx,\tilde \bs^{(1)},\bz,h) = x_1(\tilde s_1 - s_1)\Big(\frac{1}{\Delta n}\sum_{j=1}^n s_jx_j - h\Big). \label{eq:deltaH_concentration}
\end{align}
We now use similar steps as in Section~\ref{sec:subadditivitystyle} in order to evaluate the difference between the free energy associated with $\mathcal{H}(\bx,\bs, \bz,h)$ and $\mathcal{H}(\bx,\tilde \bs^{(1)},\bz,h)$. Exactly as we obtained \eqref{eq:Z_openVSclosed}, \eqref{eq:Z_openVSclosed_2}, we get
\begin{align} 
f(\bs,\bz,h) &= f(\tilde \bs^{(1)},\bz,h) - \frac{1}{n}\ln(\langle e^{-\delta \mathcal{H}(\mathbf{X},\tilde \bs^{(1)}, \bs,h)}\rangle_{\mathcal{H}}), \label{eq:ff1}\\ 
f(\tilde \bs^{(1)},\bz,h) &= f(\bs,\bz,h) - \frac{1}{n}\ln(\langle e^{\delta \mathcal{H}(\mathbf{X},\tilde \bs^{(1)}, \bs,h)}\rangle_{\tilde{\mathcal{H}}}), \label{eq:ff2}
\end{align}
where $\langle A(\mathbf{X}) \rangle_{\mathcal{H}} \defeq \mathcal{Z}(\bs,\bz,h)^{-1}\int d\bx A(\bx) P_0(\bx)\exp(-\mathcal{H}(\bx,\bs,\bz,h))$ is the expectation w.r.t the posterior associated with $\mathcal{H}(\bx,\bs,\bz,h)$ (previously denoted $\langle A(\mathbf{X}) \rangle_h$), and similarly, $\langle A(\mathbf{X}) \rangle_{\tilde{\mathcal{H}}}$ is the the expectation w.r.t the posterior associated with $\mathcal{H}(\bx,\tilde \bs^{(1)},\bz,h)$. Combining these two identites and using the convexity of the exponential, we get
\begin{align} \label{eq:sandwich_tilde_concentration}
f(\tilde \bs^{(1)},\bz,h) + \frac{\langle \delta \mathcal{H}(\mathbf{X},\tilde \bs^{(1)}, \bs,h)\rangle_{\mathcal{H}}}{n} \le f(\bs,\bz,h) \le f(\tilde \bs^{(1)},\bz,h) + \frac{\langle \delta \mathcal{H}(\mathbf{X},\tilde \bs^{(1)}, \bs,h)\rangle_{\tilde{\mathcal{H}}}}{n}.
\end{align}
Let us now estimate $\langle \delta \mathcal{H}(\mathbf{X},\tilde \bs^{(1)}, \bs)\rangle_{\mathcal{H}}/n$. From \eqref{eq:deltaH_concentration} we get
\begin{align}
\frac{\langle \delta \mathcal{H}(\mathbf{X},\tilde \bs^{(1)}, \bs)\rangle_{\mathcal{H}}}{n} = \frac{\tilde s_1-s_1}{n}\Big(\frac{1}{\Delta n} \sum_{j=1}^n s_j \langle X_1 X_j\rangle_{\mathcal{H}} - h \langle X_1\rangle_{\mathcal{H}}\Big).
\end{align}
Using that the prior $P_0$ has bounded support, the expectations appearing in the last equality are bounded as the signal $\bs, \tilde\bs$ components. Thus $\langle \delta \mathcal{H}(\mathbf{X},\tilde \bs^{(1)}, \bs)\rangle_{\mathcal{H}}/n = \mathcal{O}(1/n)$. By the same arguments, $\langle \delta \mathcal{H}(\mathbf{X},\tilde \bs^{(1)}, \bs)\rangle_{\mathcal{\tilde H}}/n = \mathcal{O}(1/n)$ as well, proving the result using \eqref{eq:sandwich_tilde_concentration}.
\end{proof}
As the free energy $f(\bs,\bz,h)$ verifies the bounded difference property, McDiarmid's inequality [\cite{McDiarmid,boucheron2004concentration}] implies the following corollary.
\begin{corollary} \label{cor:mcdiarmid}
Fix a noize realization $\bz$ and call $C \defeq \sum_{i=1}^n \max_{\bs, \tilde \bs^{(i)}}(f(\bs,\bz,h) - f(\tilde \bs^{(i)},\bz,h) )^2$ where the max is taken over signals drawn from $P_0$. The free energy $f(\bs,\bz,h)$ verifies the following inequality for any $\bs$, $r>0$
\begin{align}
P(|f(\bs,\bz,h) - \mathbb{E}_{\bS}[f(\bS,\bz,h)]| \ge r) \le 2e^{-\frac{2r^2}{C}}.
\end{align}
\end{corollary}
From this inequality, we can estimate the order of the fluctuations of the free energy.
\begin{corollary} \label{cor:fs_minus_meanfs_small}
Fix $\bz$ and call $l \defeq \max_{\bs} |f(\bs,\bz,h) - \mathbb{E}_{\bS}[f(\bS,\bz,h)] |$, where the maximum is taken over all $\bS \sim P_0$. Then for any $\beta>0$, the free energy $f(\bs,\bz,h)$ verifies
\begin{align}
\mathbb{E}_{\bS}[|f(\bS,\bz,h) - \mathbb{E}_{\bS}[f(\bS,\bz,h)] | ] = \mathcal{O}(n^{-2\beta} + e^{-n^{1-2\beta}}(l^2 + n^{-2\beta})).
\end{align}
\end{corollary}
\begin{proof}
Let us bound the l.h.s of the previous equality. Call $b = |f(\bs,\bz,h) - \mathbb{E}_{\bS}[f(\bS,\bz,h)] |$ a random variable of $\bs$ ($\bz$ is fixed). Then
\begin{align}
\mathbb{E}_{\bS}[b] &= \int_{0}^r b P(b) db + \int_{r}^l b P(b) db \nonumber \\
&\le \int_{0}^r b \,db + \int_{r}^l b P(b \ge r) db \le \frac{r^2}{2} + e^{-\frac{2r^2}{C}}(l^2-r^2),
\end{align}
where we have used Corollary~\ref{cor:mcdiarmid} for the last inequality. Lemma~\ref{lemma:bounded_diff_prop} implies that the constant $C$ appearing in Corollary~\ref{cor:mcdiarmid} is $\mathcal{O}(1/n)$. Choosing $r=n^{-\beta}$ with $\beta>0$, the result follows.
\end{proof}
Let us use the shorthand notation $f_h \defeq f(\bs,\bz,h)$, $\bar f_h\defeq \mathbb{E}_{\bS}[f(\bS,\bz,h)]$. The aim now is to estimate the fluctuations of the averaged overlap. By definition of $f_h$, using \eqref{eq:perturbed_hamiltonian} and the dominated convergence theorem we obtain 
\begin{align}
\langle q \rangle_h - \mathbb{E}_{{\bS}}[\langle q \rangle_h] = \frac{d f_h}{dh} - \frac{d\bar f_h}{dh}. \label{eq:q_f_relation}
\end{align}
The concavity of the free energy in $h$ (Lemma~\ref{lemma:perturbed_energy_concave}) allows to write the following inequalities for any $\delta >0$.
\begin{align}
&\frac{d f_h}{dh} - \frac{d\bar f_h}{dh} \le \frac{f_{h-\delta}-f_h}{\delta} - \frac{d\bar f_h}{dh} \le \frac{f_{h-\delta} - \bar f_{h-\delta}}{\delta} - \frac{f_{h} - \bar f_{h}}{\delta} + \frac{d\bar f_{h-\delta}}{dh} - \frac{d\bar f_h}{dh},  \label{eq:firstBound_df}\\
&\frac{d f_h}{dh} - \frac{d\bar f_h}{dh} \ge \frac{f_{h+\delta} - \bar f_{h+\delta}}{\delta} - \frac{f_{h} - \bar f_{h}}{\delta} + \frac{d\bar f_{h+\delta}}{dh} - \frac{d\bar f_h}{dh}. \label{eq:secondBound_df}
\end{align}
Note that the difference between the derivatives appearing here cannot be considered small as at the first order transition point, the derivative jumps. We now have all the necessary tools to show the second concentration lemma.
\begin{lemma}[Concentration of $\langle q\rangle_h$]\label{lemma:concentration_meanq}
For any $a >\epsilon>0$ fixed and $n$ large enough
\begin{align}
\int_{\epsilon}^{a} dh \mathbb{E}_{{\bS}, {\bZ}} [ ( \langle q\rangle_h - \mathbb{E}_{{\bS}}[\langle q \rangle_{h} ])^2  ] = \mathcal{O}(n^{-\frac{1}{8}}).
\end{align}
\end{lemma}
\begin{proof}
Combining \eqref{eq:firstBound_df} and \eqref{eq:secondBound_df}, we can assert that there exists some $h_*$ such that
\begin{align}
\int_{\epsilon}^{a} dh \mathbb{E}_{\bS,\bZ}[|\langle q \rangle_h - \mathbb{E}_{{\bS}}[\langle q \rangle_h]|] \le \frac{1}{\delta} \int_{\epsilon}^{a} dh\mathbb{E}_{\bS,\bZ}[f_{h_*} - \bar f_{h_*}] + \mathbb{E}_{\bZ}[\bar f_{a-\delta} - \bar f_{a}]- \mathbb{E}_{\bZ}[\bar f_{\epsilon-\delta} -  \bar f_{\epsilon}], \nonumber
\end{align}
where we used \eqref{eq:q_f_relation} to replace the l.h.s of the inequalities. Let us choose $\delta = n^{-\alpha}, \alpha>0$. Now using Corollary~\ref{cor:fs_minus_meanfs_small} and choosing $a,\epsilon$ small enough, we obtain that the integral appearing in the r.h.s of the last inequality is $\mathcal{O}(n^{\alpha-2\beta} + \exp(-n^{1-2\beta})(l^2n^{\alpha} + n^{\alpha-2\beta}))$. Remains the two other terms. By the remainder theorem, there exists $\tilde h$ such that
\begin{align}
\bar f_{a-\delta} - \bar f_{a} = \delta \frac{d\bar f_{h}}{dh}\Big|_{a-\delta} + \mathcal{O}\Big(\delta^2 \frac{d^2\bar f_{h}}{dh^2}\Big|_{\tilde h} \Big). \label{eq:fadelta_minus_fa}
\end{align}
From the fact that the prior has bounded support, the overlap $q$ has finite expectation and variance, thus from \eqref{eq:perturbed_energy_derivative1} the first derivative of $\bar f_h$ is bounded by a constant independent of $n$, while \eqref{eq:perturbed_energy_derivative2} implies that the second derivative is $\mathcal{O}(n)$. Thus \eqref{eq:fadelta_minus_fa} implies that $\bar f_{a-\delta} - \bar f_{a} = \mathcal{O}(n^{-\alpha} + n^{1-2\alpha})$. The same arguments remain valid for the term $f_{\epsilon-\delta} -  \bar f_{\epsilon}$. Combining these results, we get that for any $\alpha, \beta >0$
\begin{align}
\int_{\epsilon}^{a} dh \mathbb{E}_{\bS,\bZ}[|\langle q \rangle_h - \mathbb{E}_{{\bS}}[\langle q \rangle_h]|] = \mathcal{O}(n^{\alpha-2\beta} + e^{-n^{1-2\beta}}(l^2n^{\alpha} + n^{\alpha-2\beta}) + n^{-\alpha} + n^{1-2\alpha}).\nonumber
\end{align}
Notice that Lemma~\ref{lemma:bounded_diff_prop} implies straightforwardly that $l = \mathcal{O}(1)$. Now choose for example $\alpha = 5/8$ and $\beta = 3/8$. Then keeping only the dominating term as $n\to\infty$, we obtain
\begin{align}
\int_{\epsilon}^{a} dh \mathbb{E}_{{\bS}, {\bZ}} [ | \langle q\rangle_h - \mathbb{E}_{{\bS}}[\langle q \rangle_{h} ]|  ] = \mathcal{O}(n^{-\frac{1}{8}}).
\end{align}
The last step is to go from the concentration in the absolute value sense that we just obtained to the concentration in the square sense. Recall that the overlap is bounded independently of $n$ as $P_0$ has bounded support. Thus $| \langle q\rangle_h - \mathbb{E}_{{\bS}}[\langle q \rangle_{h} ] | = \mathcal{O}(1)$ for any $h$ and disorder realization, which implies
\begin{align}
\int_{\epsilon}^{a} dh\mathbb{E}_{{\bS}, {\bZ}} [ ( \langle q\rangle_h - \mathbb{E}_{{\bS}}[\langle q \rangle_{h} ] )^2 ] &= \int_{\epsilon}^{a} dh\mathbb{E}_{{\bS}, {\bZ}} [ | \langle q\rangle_h - \mathbb{E}_{{\bS}}[\langle q \rangle_{h} ] || \langle q\rangle_h - \mathbb{E}_{{\bS}}[\langle q \rangle_{h} ] | ] \nonumber \\
&= \mathcal{O}\Big(\int_{\epsilon}^{a} dh\mathbb{E}_{{\bS}, {\bZ}} [ | \langle q\rangle_h - \mathbb{E}_{{\bS}}[\langle q \rangle_{h} ] | ] \Big),
\end{align}
which ends the proof.
\end{proof}
\subsection{Concentration of $\mathbb{E}_{{\bS}}[\langle q \rangle_h]$ on $\mathbb{E}_{{\bS}, {\bZ}}[\langle q \rangle_h]$}
We finally prove the last concentration property of the overlap. The strategy is the following. We will show that on a properly defined ensemble $\mathcal{Y}$ of noize realizations where these are bounded, the free energy verifies the bounded difference property which will allow to use the same strategy as the previous section~\ref{subsec:concetration2}. The probability of the complementary set $\mathcal{Y}^{\rm c}$ is negligible as the signal size increases, which will allow to show the desired concentration. Let us start defining $\mathcal{Y}\defeq \{{\bZ} | \,|z_{ij}| \le n^{y} \ \forall \ i,j \in\{1:n\}\}$ for some $y>0$ that is to be fixed later on. Call $\gamma \defeq P(\bz \notin \mathcal{Y})$. We can write 
\begin{align}
\mathbb{E}_{{\bZ}}\big[|\mathbb{E}_{{\bS}}[\langle q \rangle_h] - \mathbb{E}_{{\bS}, {\bZ}}[\langle q \rangle_h]|\big]=\ &(1-\gamma)\mathbb{E}_{{\bZ}\in \mathcal{Y}}\big[|\mathbb{E}_{{\bS}}[\langle q \rangle_h] - (1-\gamma)\mathbb{E}_{{\bS}, {\bZ}\in \mathcal{Y}}[\langle q \rangle_h]  - \gamma\mathbb{E}_{{\bS}, {\bZ}\notin \mathcal{Y}}[\langle q \rangle_h] | \big]  \nonumber\\
&+ \gamma\mathbb{E}_{{\bZ}\notin \mathcal{Y}}\big[|\mathbb{E}_{{\bS}}[\langle q \rangle_h] - (1-\gamma)\mathbb{E}_{{\bS}, {\bZ}\in \mathcal{Y}}[\langle q \rangle_h] - \gamma\mathbb{E}_{{\bS}, {\bZ}\notin \mathcal{Y}}[\langle q \rangle_h] | \big] \nonumber \\
%
% \le\ &(1-\gamma)\mathbb{E}_{{\bZ}\in \mathcal{Y}}\big[|\mathbb{E}_{{\bS}}[\langle q \rangle_h] - (1-\gamma)\mathbb{E}_{{\bS}, {\bZ}\in \mathcal{Y}}[\langle q \rangle_h] | \big]  \nonumber\\
% &+ \gamma\mathbb{E}_{{\bZ}\notin \mathcal{Y}}\big[|\mathbb{E}_{{\bS}}[\langle q \rangle_h] - (1-\gamma)\mathbb{E}_{{\bS}, {\bZ}\in \mathcal{Y}}[\langle q \rangle_h] | \big] + \gamma \nonumber \\
%
\le \ &\mathbb{E}_{{\bZ}\in \mathcal{Y}}\big[|\mathbb{E}_{{\bS}}[\langle q \rangle_h] - \mathbb{E}_{{\bS}, {\bZ}\in \mathcal{Y}}[\langle q \rangle_h] | \big]  + \mathcal{O}(\gamma), \label{eq:meanoverlap_dividedYnotY}
\end{align}
where we used the triangle inequality and the fact that the $\langle q\rangle_h=\mathcal{O}(1)$ uniformly in $n$ as $P_0$ has bounded support independently of $n$. Let us estimate $\gamma = 1 - P(\bz \in \mathcal{Y})$. As the noise components $Z_i$ are standardized random Gaussian variables, we have
\begin{align}
P(\bz \in \mathcal{Y}) = \Big(\int_{-n^y}^{n^y} \frac{e^{-\frac{z^2}{2}}}{\sqrt{2\pi}} dz \Big)^{n^2} = \Big({\rm erf}\Big(\frac{n^y}{\sqrt{2}}\Big)\Big)^{n^2} = \Big(1-\frac{2e^{-n^{2y}}}{n^y\sqrt{\pi}} + \mathcal{O}(e^{-n^{2y}}n^{-3y} \Big) \Big)^{n^2},
\end{align}
where the last equality comes from a canonical approximation of the error function ${\rm erf}(x)$ as $x\to\infty$. After Taylor expansion as $n \to \infty$, we deduce
\begin{align}
\gamma = \frac{2}{\sqrt{\pi}}e^{-n^{2y}}n^{2-y} + \mathcal{O}(e^{-n^{2y}}n^{2-3y}) = \mathcal{O}(e^{-n^{2y}}n^{2-y}), \label{eq:PznotinY_verysamll}
\end{align}
which goes to zero super exponentially as $n\to\infty$. Now we use similar steps as in the previous section. The perturbed noize is $\tilde \bz^{(ij)}$, with all its components being the same as the ones of $\bz$ except its component $(ij)$ that is $\tilde z_{ij}$. The perturbed system corresponds now to the Hamiltonian \eqref{eq:perturbed_hamiltonian} evaluated at this perturbed noize.
\begin{lemma}[Bounded difference property] \label{lemma:bounded_diff_prop_2}
Assume that both $\bz, \tilde \bz^{(ij)}\in \mathcal{Y}$. Then the free energy of the perturbed system verifies the bounded difference property w.r.t the noize
\begin{align}
|\mathbb{E}_{\bS}[f(\bS,\bz,h)] - \mathbb{E}_{\bS}[f(\bS,\tilde \bz^{(ij)},h)]| = \mathcal{O}(n^{y-3/2}) \ \forall \ i,j \in \{1:n\}.
\end{align}
\end{lemma}
\begin{proof}
The proof works as for Lemma~\ref{lemma:bounded_diff_prop}. The perturbation of the Hamiltonian \eqref{eq:perturbed_hamiltonian} is
\begin{align}
\delta \mathcal{H}(\bx,\tilde \bz^{(ij)}, \bz,h) \defeq \mathcal{H}(\bx,\bs, \bz,h) - \mathcal{H}(\bx,\bs,\tilde\bz^{(ij)},h) = \frac{\tilde z_{ij} - z_{ij}}{\sqrt{n\Delta}}x_ix_j. \label{eq:deltaH_concentration_2}
\end{align}
As in the previous section, we evaluate the difference between the free energy associated with $\mathcal{H}(\bx,\bs, \bz,h)$ and $\mathcal{H}(\bx,\bs,\tilde \bz^{(ij)},h)$. Similar steps as \eqref{eq:ff1}, \eqref{eq:ff2} lead to
\begin{align} \label{eq:sandwich_tilde_concentration_2}
\mathbb{E}_{\bS}[f(\bS,\tilde\bz^{(ij)},h)] + \frac{\langle \delta \mathcal{H}(\mathbf{X},\tilde \bz^{(ij)}, \bz,h)\rangle_{\mathcal{H}}}{n} &\le \mathbb{E}_{\bS}[f(\bS,\bz,h)] \nonumber \\&\le \mathbb{E}_{\bS}[f(\bS,\tilde \bz^{(ij)},h)] + \frac{\langle \delta \mathcal{H}(\mathbf{X},\tilde \bz^{(ij)}, \bz,h)\rangle_{\tilde{\mathcal{H}}}}{n}.
\end{align}
where $\langle A(\mathbf{X}) \rangle_{\mathcal{H}}$ is the expectation w.r.t the posterior associated with $\mathcal{H}(\bx,\bs,\bz,h)$, and similarly, $\langle A(\bX) \rangle_{\tilde{\mathcal{H}}}$ is the the expectation w.r.t the posterior associated with $\mathcal{H}(\bx,\bs,\tilde \bz^{(ij)},h)$. From \eqref{eq:deltaH_concentration_2} we get
\begin{align}
\frac{\langle \delta \mathcal{H}(\mathbf{X},\tilde \bz^{(ij)}, \bz)\rangle_{\mathcal{H}}}{n} = \frac{\tilde z_{ij} - z_{ij}}{n^{3/2}\sqrt{\Delta}}\langle X_iX_j \rangle_{\mathcal{H}} = \mathcal{O}(n^{y-3/2}), 
\end{align}
where we used that $P_0$ has bounded support, which makes $\langle X_iX_j \rangle_{\mathcal{H}}=\mathcal{O}(1)$. Furthermore, as both $\bz, \tilde \bz^{(ij)} \in \mathcal{Y}$, then $\tilde z_{ij} - z_{ij} = \mathcal{O}(n^y)$. The same arguments apply when evaluating $\langle \delta \mathcal{H}(\mathbf{X},\tilde \bz^{(ij)}, \bz)\rangle_{\mathcal{\tilde H}}$. Thus using \eqref{eq:sandwich_tilde_concentration_2}, the result follows.
\end{proof}
McDiarmid's inequality then provides the following corollary.
\begin{corollary} \label{cor:mcdiarmid_2}
Call $K \defeq \sum_{i,j=1}^n \max_{\bz, \tilde \bz^{(ij)}}(\mathbb{E}_{\bS}[f(\bS,\bz,h)] - \mathbb{E}_{\bS}[f(\bS,\tilde \bz^{(ij)},h) ] )^2$ where 
the max is taken over noize realizations $\in \mathcal{Y}$. Then the free energy verifies the following inequality for any $r>0$
\begin{align}
P(|\mathbb{E}_{\bS}[f(\bS,\bz,h)] - \mathbb{E}_{\bS,{\bZ}\in \mathcal{Y}}[f(\bS,\bZ,h)]| \ge r) \le 2e^{-\frac{2r^2}{K}}.
\end{align}
\end{corollary}
Notice from Lemma~\ref{lemma:bounded_diff_prop_2} that $K=\mathcal{O}(n^{2y-1})$. Using the same proof as for Corollary~\ref{cor:fs_minus_meanfs_small} but considering this time $\mathbb{E}_{\bZ\in \mathcal{Y}}[|\mathbb{E}_{\bS}[f(\bS,\bZ,h)] - \mathbb{E}_{\bS,\bZ\in \mathcal{Y}}[f(\bS,\bZ,h)] |]$, we obtain the next corollary.
\begin{corollary} \label{cor:fs_minus_meanfs_small_2}
Call $u \defeq \max_{\bz \in \mathcal{Y}} |\mathbb{E}_{\bS}[f(\bS,\bz,h)] - \mathbb{E}_{\bS,\bZ\in \mathcal{Y}}[f(\bS,\bZ,h)] |$. Then for any $\beta>0$, the average free energy $\mathbb{E}_{\bS}[f(\bS,\bz,h)]$ verifies
\begin{align}
&\mathbb{E}_{\bZ\in \mathcal{Y}}[|\mathbb{E}_{\bS}[f(\bS,\bZ,h)] - \mathbb{E}_{\bS,\bZ\in \mathcal{Y}}[f(\bS,\bZ,h)] | ] =\mathcal{O}(n^{-2\beta} + e^{-n^{1-2(\beta+y)}}(u^2 +  n^{-2\beta})).
\end{align}
\end{corollary}
Now call $f_h\defeq \mathbb{E}_{\bS}[f(\bS, \bz, h)]$ and $\bar f_h\defeq \mathbb{E}_{\bS, \bZ\in\mathcal{Y}}[f(\bS, \bZ, h)]$. By dominated convergence theorem, Lemma~\ref{lemma:perturbed_energy_concave} remains valid for $f_h, \bar f_h$, \eqref{eq:firstBound_df}, \eqref{eq:secondBound_df} as well and \eqref{eq:q_f_relation} becomes with these new definitions
\begin{align}
\mathbb{E}_{{\bS}}[\langle q \rangle_h] - \mathbb{E}_{{\bS},{\bZ}\in\mathcal{Y}}[\langle q \rangle_h] = \frac{d f_h}{dh} - \frac{d\bar f_h}{dh}. \label{eq:q_f_relation_2}
\end{align}
We can now show the last concentration property of the overlap.
\begin{lemma}[Concentration of $\mathbb{E}_{\bS}{[}\langle q\rangle_h{]}$]\label{lemma:concentration_mean2}
For any $a >\epsilon>0$ fixed and $n$ large enough
\begin{align}
\int_{\epsilon}^{a} dh \mathbb{E}_{{\bZ}} [ ( \mathbb{E}_{{\bS}}[\langle q \rangle_{h} ] - \mathbb{E}_{{\bS,\bZ}}[\langle q \rangle_{h} ])^2  ] = \mathcal{O}(n^{-\frac{1}{8}}).
\end{align}
\end{lemma}
\begin{proof}
The proof goes along the same lines as the one of Lemma~\ref{lemma:concentration_meanq}, and is based on Corollary~\ref{cor:fs_minus_meanfs_small_2}, \eqref{eq:q_f_relation_2} and \eqref{eq:firstBound_df}, \eqref{eq:secondBound_df}. Using \eqref{eq:meanoverlap_dividedYnotY} combined with \eqref{eq:PznotinY_verysamll}, one obtains that for small enough $a,\epsilon$ and any positive $\alpha$ and $\beta$
\begin{align}
&\int_{\epsilon}^{a} dh \mathbb{E}_{\bZ}[|\mathbb{E}_{\bS}[\langle q \rangle_h] - \mathbb{E}_{{\bS},\bZ}[\langle q \rangle_h]|]\nonumber \\
= \, &\mathcal{O}(n^{\alpha-2\beta} + e^{-n^{1-2(\beta+y)}}(u^2n^{\alpha} + n^{\alpha-2\beta}) + n^{-\alpha} + n^{1-2\alpha} +e^{-n^{2y}}n^{2-y}).
\end{align}
Lemma~\ref{lemma:bounded_diff_prop_2} implies $u = \mathcal{O}(n^{y+1/2})$. Choosing, $\alpha = 5/8$, $\beta = 3/8$ and $y=1/16$, the remaining dominating term as $n\to\infty$ in the last equality is $\mathcal{O}(n^{-\frac{1}{8}})$. Going from the this concentration to the one in the square sense works like in the proof of Lemma~\ref{lemma:concentration_meanq}.
\end{proof}
