# Supplementary material for: Rank-one matrix estimation: analysis of algorithmic and information theoretic limits by the spatial coupling method
Source: arXiv:1812.02537 source file (2018-12-06)
Supplement: Supplementary file 3 [file appendix_concentration_M.tex]

\appendix \label{app:concentration_M}
\section{Concentration of the overlap}
In order to show the connection between the matrix-mmse and the vector-mmse, it turns out that we need some concentration properties on the overlap $q \defeq 1/n \sum_i x_i^{(1)}x_i^{(2)}$ between the two independent replicas $x_i^{(1)}$ and $x_i^{(2)}$. For this end, we consider a \emph{perturbed} system with the following Hamiltonian
\begin{align}\label{eq:perturbed_hamiltonian}
\mathcal{H}(\bx,h) &= \frac{1}{\Delta} \sum_{1 \le i\le j\le n}\bigg[ \frac{x_{i}^2x_{j}^2}{2n} -  \frac{s_{i}s_{j}x_{i}x_{j}}{n} - \frac{x_{i}x_{j}z_{i j} \sqrt{\Delta}}{\sqrt{n}} \bigg] + h \sum_i x_i^{(1)}x_i^{(2)},
\end{align}
where a perturbation term $h \sum_i x_i^{(1)}x_i^{(2)}$ is added to the original Hamiltonian (again, the dependence of the Hamiltonian on $\bs,\bz,\Delta$ and $n$ is implicit and dropped from the notation of $\mathcal{H}(\bx,h)$ for readability). Note that $\mathcal{H}(\bx,0)$ corresponds to the Hamiltonian of the original system. However, for some technical reasons that will become clear in the sequel, we work with the perturbed system (\ref{eq:perturbed_hamiltonian}) and then let $h \rightarrow 0$ at the end of the analysis.

Let $Z(h)$ be the partition function associated with $\mathcal{H}(\bx,h)$ and denote by $f_{h,n}$ the free energy of the perturbed system at fixed signal and noise realization with $f_{h,n} =  - \ln \big( Z(h) \big)/n$. Moreover, we denote by $\langle \cdot \rangle_{h}$ the expectation over the posterior distribution associated with $\mathcal{H}(\bx, h)$. Note the the perturbation term has been chosen so that the following lemma holds.
\begin{lemma}\label{lemma:pertubed_energy_concave}
$f_{h,n}$ is concave in $h$.
\end{lemma}
\begin{proof}
By using the dominated convergence theorem, one obtains the following
\begin{align}
\label{eq:perturbed_energy_derivative1}
\frac{d}{dh} f_{h,n} &=  \langle q \rangle_{h} \\
\label{eq:perturbed_energy_derivative2}
\frac{d^2}{dh^2} f_{h,n} &= - n \Big( \langle q^2 \rangle_{h} - \langle q \rangle_{h}^2 \Big) \le 0. 
\end{align}
\end{proof}
Furthermore, it turns out the the overlap $q$ satisfies some concentration properties.
\begin{lemma}\label{lemma:concentration_q}
Concentration of $q$: For any $a >\epsilon>0$ fixed
\begin{align*}
\int_{\epsilon}^{a} dh \mathbb{E} \Big[ \Big\langle \big(q - \langle q \rangle_{h} \big)^2 \Big\rangle_{h} \Big] = \mathcal{O}\Big(\frac{1}{n}\Big).
\end{align*}
\end{lemma}
\begin{proof}
\begin{align*}
\int_{\epsilon}^{a} dh \mathbb{E} \Big[ \Big\langle \big(q - \langle q \rangle_{h} \big)^2 \Big\rangle_{h} \Big]
&= \int_{\epsilon}^{a} dh \mathbb{E} \big[ \langle q^2 \rangle_{h} - \langle q \rangle_{h}^2 \big]
= - \int_{\epsilon}^{a} dh \frac{1}{n} \frac{d^2}{dh^2} \mathbb{E} \big[f_{h,n} \big]\\
&= \frac{1}{n} \Big( \frac{d}{dh} \mathbb{E} \big[f_{\epsilon,n}\big] - \frac{d}{dh} \mathbb{E} \big[f_{a,n}\big] \Big) = \mathcal{O}\Big(\frac{1}{n}\Big),
\end{align*}
where the second equality follows from (\ref{eq:perturbed_energy_derivative2}) and the dominated convergence theorem. The last equality uses the fact that the derivative of $\mathbb{E} \big[f_{h,n}\big]$ is $\mathcal{O}(1)$ for $h\ge\epsilon$, which is valid, by Nishimori condition, for all signal's prior distribution with bounded second moment
\begin{align*}
\frac{d}{dh} \mathbb{E} \big[f_{h,n}\big] =  \frac{1}{n} \sum_i \mathbb{E} \big[ \langle x_i^{(1)}x_i^{(2)} \rangle_{h} \big] = \mathbb{E} \big[ \langle s_i x_i \rangle_{h} \big] \le \mathbb{E} \big[  s_i^2 \big] = v. 
\end{align*} 
\end{proof} 
